# Supplementary material for: Fermi surface geometry and momentum dependent electron-phonon coupling drive the charge density wave in quasi-1D ZrTe$3$
Source: arXiv:2602.04534 ancillary file (2026-05-08)
Supplement: Supplementary file 1 [file SI.pdf]

# Supplementary Information for ‘Fermi surface geometry and momentum dependent electron-phonon coupling drive the charge density wave in quasi-1D ZrTe<sub>3</sub>’

Josu Diego<sup>1,\*</sup> and Matteo Calandra<sup>1,†</sup>

<sup>1</sup>*Dipartimento di Fisica, Università di Trento, Via Sommarive 14, 38123 Povo, Italy.*

## A. Convergence of the CDW phonon mode

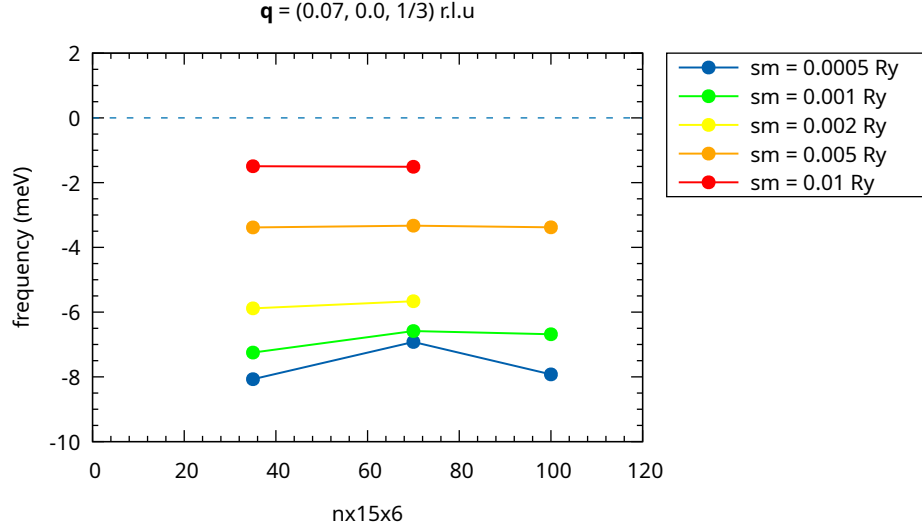

Supplementary Fig. 1. Convergence of the harmonic phonon frequency of the CDW driving mode with respect to the  $\mathbf{k}$ -point mesh ( $n \times 15 \times 6$ ) for different electronic smearing values within PBE+U. For each smearing, increasing the  $\mathbf{k}$ -point density leads to only minor changes in the phonon frequency, indicating good  $\mathbf{k}$ -point convergence. Smaller smearing values systematically yield lower phonon frequencies, consistent with enhanced Fermi surface nesting effects.

---

\* josu.diegolopez@unitn.it

† m.calandrabuonaura@unitn.it

### B. Electronic structure of the high-temperature phase

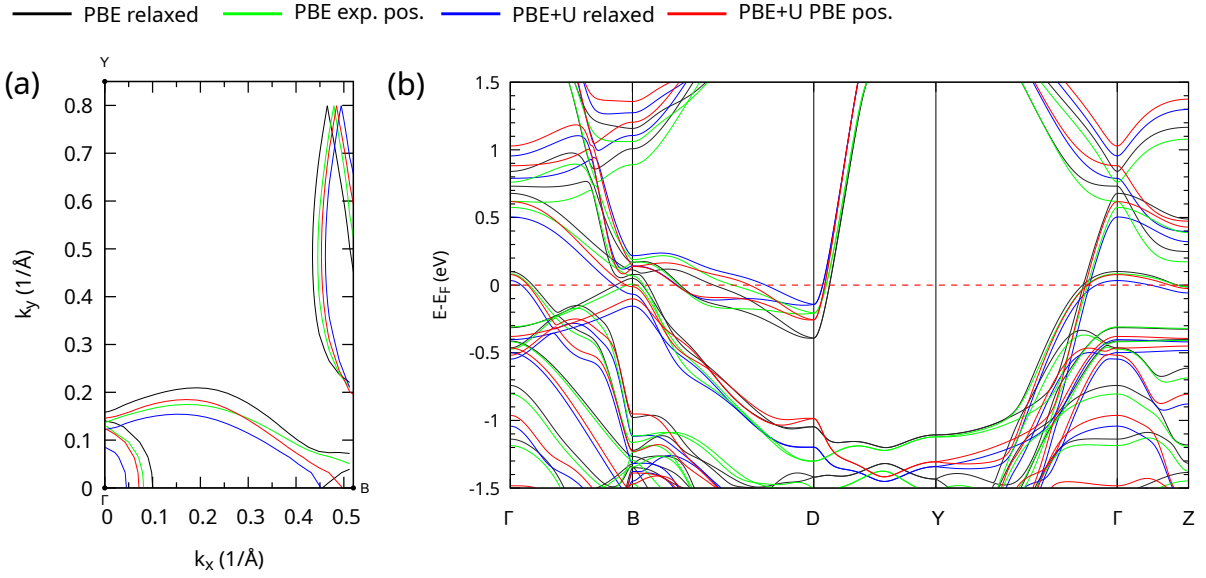

Supplementary Fig. 2. Electronic properties of the HT phase of  $\text{ZrTe}_3$ : (a) Fermi surface at  $k_z = 0$  and (b) electronic band structure for different electronic-correlation schemes (PBE and PBE+U) and internal atomic coordinates.

### C. Extended Brillouin zone analysis of the nesting function and electronic susceptibility

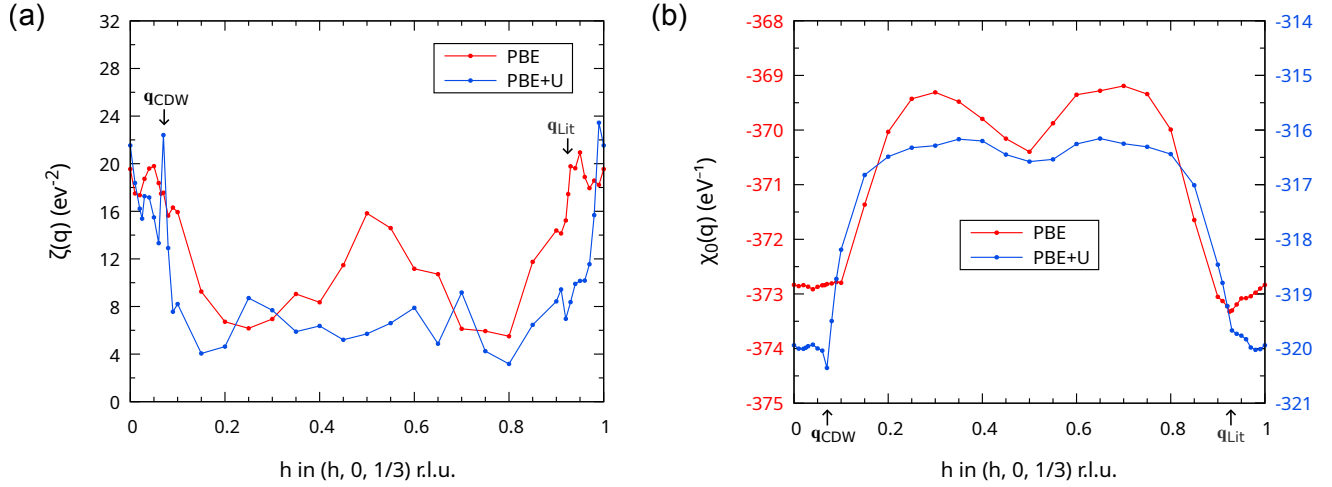

Supplementary Fig. 3. Quantities related to the non-interacting static electronic susceptibility at different levels of theory (PBE: red; PBE+U: blue), corresponding to those shown in Fig. 3 of the main text, but extended to the full momentum range. (a) Nesting function along  $(h, 0, 1/3)$  r.l.u. for  $h \in [0, 1]$ . (b) Real part of the non-interacting susceptibility in the same momentum range. Note that different y-axis scales are used in panel (b) for PBE (left, red) and for PBE+U (right, blue). Arrows in both panels indicate nesting vectors: the black arrow marks the experimental CDW, while the gray arrow corresponds to the theoretical vector reported in the literature.

In the literature, theoretical calculations at the PBE level often predict a nesting vector at  $\mathbf{q}_{\text{Lit}} = (0.93, 0, 1/3)$  r.l.u. [1, 2], which is not equivalent by symmetry to the experimental  $\mathbf{q}_{\text{CDW}} = (0.07, 0, 1/3)$  r.l.u.. In our PBE calculations with relaxed coordinates (red lines), this vector corresponds to the largest softening in  $\chi_0(\mathbf{q})$  but does not lead to a phonon instability (see 4). When DFT+U is applied, the nesting shifts to  $h = 0.07$ , in agreement with experiment.

#### D. Extended Brillouin zone analysis of the phonon dispersion

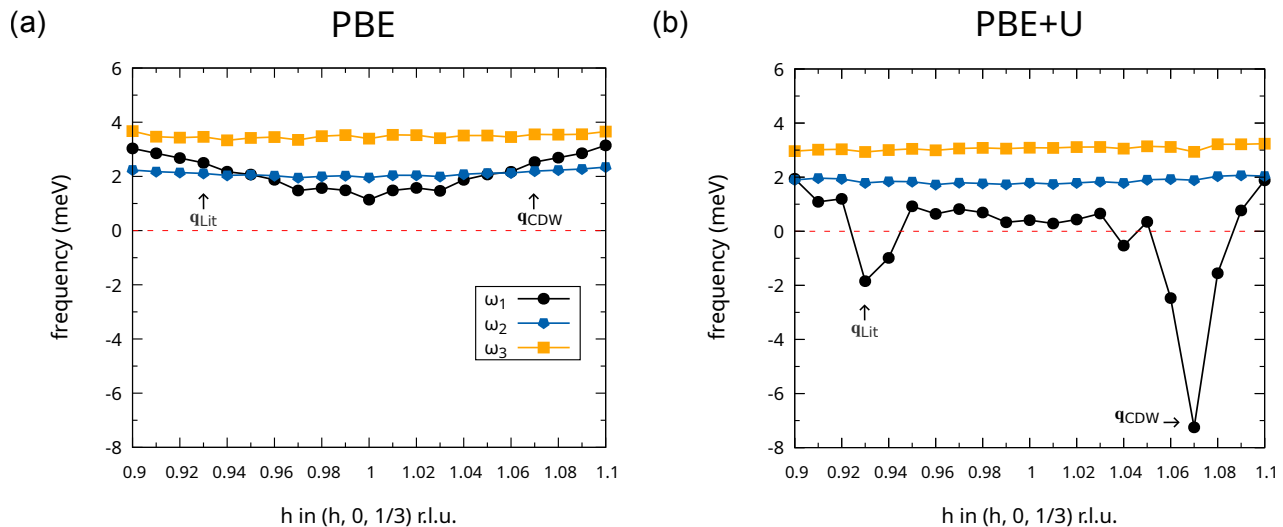

Supplementary Fig. 4. Harmonic phonon spectra of ZrTe<sub>3</sub> calculated with PBE (a) and PBE+U (b) along  $(h, 0, 1/3)$  r.l.u for  $h \in [0.90, 1.10]$ . Only acoustic modes are shown. Within PBE, no dynamical instabilities are found in this momentum range. In contrast, the PBE+U calculation reveals a pronounced instability at the experimentally observed CDW wavevector  $\mathbf{q}_{\text{CDW}}$  (black arrow), which corresponds to the physically relevant ordering vector. A secondary and significantly weaker instability is also present at  $\mathbf{q}_{\text{Lit}}$  (gray arrow), with a depth of approximately -2 meV, which is likely removed by anharmonic effects. Although the points  $h$  and  $-h$  at fixed  $q_z = 1/3$  are not symmetry-equivalent under the space group of ZrTe<sub>3</sub>, an approximate inversion-like symmetry arises in the Brillouin zone due to the presence of nearly parallel, quasi-1D Fermi surface sheets formed by closely spaced lamellae, which can be connected by small displacements in  $h$ .

- 
- [1] K. Stöwe and F. R. Wagner, J. Solid State Chem. **138**, 160 (1998).  
[2] C. Felser, E. W. Finckh, H. Kleinke, F. Rocker, and W. Tremel, J. Mater. Chem. **8**, 1787 (1998).
